# Supplementary material for: The Impact of Recommendation Systems on Opinion Dynamics: Microscopic versus Macroscopic Effects
Source: arXiv:2309.08967 source file (2023-12-07)
Supplement: Supplementary file 2 [file additional_case_study.tex]

\subsection{Does polarization penetrate through the population?}

In our second analysis, we investigate if and to what extent a polarized recommendation distribution leads to a polarized opinion distribution. For this case study, we consider a population with $\beta=0.8$ and initial opinion uniformly distributed between $-2$ and $2$. Recommender systems have, as above, exploration parameter $T\in\{1,\ldots,21\}$ and the recommendations distributed according to a mixture of Gaussians with standard deviation $0.1$ and mean $\pm \alpha/2$, with $\alpha\in\{0,0.1,\ldots,2\}$ (see~\cref{.}). For each setting, we perform 20 exploration cycles. 
This way, $\weightopinion^{T-1}$, the key quantity revealed by our first case study, varies between $0.01$ and $1.0$, and the distance between the two modes of the polarized recommendation distribution is $\alpha$.

\begin{figure}[bt]
    \centering 
    \begin{tikzpicture}
    \begin{axis}[name=one,
                 colorbar, colorbar style={width=0.2cm,xshift=-0.3cm},
                 width=4.4cm, height=4.4cm,
                 view={0}{90},
                 point meta min=0, %point meta max=0.7,
                 xlabel={$\weightopinion^{T-1}$},
                 %xmin=1, xmax=21,
                 %xtick={1,6,...,19},
                 ylabel={$\alpha$}, ylabel style={yshift=-0.15cm},
                 ymin=0, ymax=2,
                 ytick={0,0.4,...,2},
                 shader=interp,
                 colormap/viridis,
                 %mesh/ordering=x varies,
                 ]
    \addplot3[surf,mesh/cols=20] table [x expr=\thisrowno{0}, y expr=\thisrowno{1}, z expr=\thisrowno{2}, col sep=comma] {figures/dpol.csv}; 
    \end{axis}
    \end{tikzpicture}
    \caption{\ldots For this simulation, we use the same setting as in~\cref{subsec:model:simulation}.}
    \label{fig:noexploration}
\end{figure}
